# Supplementary material for: Learning to refine domain knowledge for biological network inference
Source: arXiv:2410.14436 source file (2024-10-18)
Supplement: Supplementary file 1 [file 6-appendix.tex]

%%%%%%%%%%%%%%%%%%%%%%%%%%%%%%%%%%%%%%%%%%%%%%%%%%%%%%%%%%%%%%%%%%%%%%%%%%%%%%%
%%%%%%%%%%%%%%%%%%%%%%%%%%%%%%%%%%%%%%%%%%%%%%%%%%%%%%%%%%%%%%%%%%%%%%%%%%%%%%%
% APPENDIX
%%%%%%%%%%%%%%%%%%%%%%%%%%%%%%%%%%%%%%%%%%%%%%%%%%%%%%%%%%%%%%%%%%%%%%%%%%%%%%%
%%%%%%%%%%%%%%%%%%%%%%%%%%%%%%%%%%%%%%%%%%%%%%%%%%%%%%%%%%%%%%%%%%%%%%%%%%%%%%%
\newpage
\appendix

\section{Experimental details}
\label{sec:experiment-appendix}

\subsection{Synthetic data generation}
\label{subsec:causal-mechanisms}

\subsection{Baseline details}
\label{subsec:baselines}

We considered the following baselines, run using official implementations published by the authors.

\textbf{\textsc{Dcdi}} \citep{dcdi}

\textbf{\textsc{Dcd-Fg}} \citep{dcdfg}

\subsection{Neural network design}
\label{subsec:hyperparameters}

\subsection{Training and hardware details}
\label{subsec:pretraining}

\section{Additional analyses}
\label{sec:more-experiments}
